# Supplementary material for: Coherent Tunneling and Strain Sensitivity of an All Heusler Alloy Magnetic Tunneling Junction: A First-Principles Study
Source: arXiv:2309.09755 source file (2023-09-18)
Supplement: Supplementary file 1 [file Supple.pdf]

# Coherent Tunneling and Strain Sensitivity of All−Heusler Alloy Magnetic Tunneling Junction: A First-Principles Study

Joydipto Bhattacharya[1,2], Ashima Rawat[3], Ranjit Pati[3], Aparna Chakrabarti[†1,2], Ravindra Pandey[3]
[1]*Raja Ramanna Centre for Advanced Technology, Indore 452013, India*
[2]*Homi Bhabha National Institute, Training School Complex, Anushakti Nagar, Mumbai 400094, India and*
[3]*Department of Physics, Michigan Technological University, Houghton, Michigan 49931, USA*

Table 1 summarizes the calculated physical properties of the bulk electrode material $Co_2MnSb$. Consistent with the Slater-Pauling formula, $Co_2MnSb$ exhibits HM behavior with a total magnetic moment of 6 $\mu_B$ per formula unit and a predicted high Curie temperature. DFT calculations demonstrate that the HM character is defect tolerant, making it an attractive candidate for spin-injecting devices. However, some disordered states have been found to exceed the predicted magnetic moment, suggesting a possible higher Curie temperature than the parent compound. The spin-resolved band structure (Figure S1) confirms the HM behavior with a gap of 0.42 eV in the minority spin channel. The symmetry of the bands crossing the Fermi energy ($E_F$) is also important to understand, and from the symmetry analyses, it is confirmed that in the majority spin channel, the lower energy band crossing the $E_F$ possesses a $\Delta_1$ symmetry, while the doubly degenerate higher energy bands correspond to the $\Delta_5$ symmetry. This orbital symmetry character is similar to that of $Co_2MnSi$ alloy[4], which has been extensively studied as an electrode material for MTJ systems. The significance of the presence of bands with $\Delta_1$ symmetry will be discussed later.

Understanding how bi-axial strain affects the electronic and magnetic properties of electrode materials is crucial, particularly in investigating the heterostructure properties where strain can arise from the substrate or metal-insulator interfaces. In this study, we considered both compression and expansion of the in-plane lattice parameters (a and b), and the geometry was not allowed to relax. The in-plane strain with respect to the undistorted structure is summarized in Table S3, and the spin-polarized DOS with compressive and tensile strain is shown in Figure S2. We observed that the HM property is maintained over the entire range of tensile strain, and the center of the HM gap shifts towards the conduction band, such that the position of the Fermi level ($E_F$) lies within the gap. However, compressive bi-axial strain appeared to destroy the HM property, as it caused the minority spin states to shift towards $E_F$, thereby reducing both the spin polarization value at $E_F$ and the magnetic moment (Table S3).

We further investigated the effect of bi-axial strain on the majority and minority spin band structure along the Γ to X direction (i.e., along the propagation direction) in Figures S3, S4, and S5. Rigid shift of the bands with no significant impact on the band dispersion has been observed. Given that $Co_2MnSb$ loses its HM properties under compressive bi-axial strain, we examine the orbital character of the bands near $E_F$ in the minority spin channel. In Figure S3, we present the contribution of the $\Delta_1$ orbitals to the minority spin bands under compressive bi-axial strain. We observe that the bands crossing at $E_F$ have a dominant $\Delta_1$ character, which is likely to contribute to the electron transmission across the junction. This could significantly affect the TMR value, as we will discuss later in this paper.

*.0.1. Electronic and Magnetic properties of Surface*

The performance of spintronic devices heavily relies on the surface properties of electrode materials. In this study, we first investigated the electronic structure properties of various $Co_2MnSb$ surface terminations. We generated three types of surfaces by simulating the cleavage of the optimized bulk structure along the (001) crystal orientation, as shown in Figure S7: naturally terminating surfaces with Co-Co and Mn-Sb terminations, and an off-stoichiometric surface with a Mn-rich (Mn-Mn) termination obtained by replacing one of the surface Sb atoms with a Mn atom. To determine the relative stability of the different surfaces, we calculated their surface free energies and summarized the results in Table S3. Our results indicate that the Co-Co terminated surface has the lowest surface energy. However, the other two surface terminations exhibit negative surface energy, suggesting the possibility that they can be synthesized under non-equilibrium conditions, even though the Co-Co terminated surface may be easier to form.

To identify the surface with the highest SP, the electronic structure of various surfaces has been investigated, as shown in Figure S7. The results reveal that the Mn-Sb and Mn-Mn interfaces preserve the half-metallic (HM) property of the bulk, while the Co-Co surface destroys the HM character. The stronger localization of the *d*-electrons as compared to bulk, can be seen in S7, which leads to the increase in magnetic moments of the surface atoms, as shown in Table S3. Moreover, an increase in the exchange splitting energy for the surface atoms compared to the bulk is observed in Figure S7, resulting in larger surface magnetic moments.

The Mn-Sb and Mn-Mn terminated surfaces were found to possess high surface SP and thus, we further

Table S1. Calculated bulk properties of the relevant full and half Heusler alloys: equilibrium lattice parameter a in Å, band gap energy from the Fermi level $E_g$ (HM written in brackets indicates that the material is half-metallic) in eV, Spin magnetic moment $M_S$ given in $\mu_B$ per f.u. In the last column, we report the symmetries of the bands that cross the $E_F$ of the electrode and the symmetries associated to the valence band maxima (VBM) and conduction band minima (CBM) of the spacer materials, respectively. Values from the literature are given inside brackets, with the references mentioned in the superscript.

| Material | a | $E_g$ | $M_S$ | Role | Band Symmetry |
|---|---|---|---|---|---|
| | | | | | VBM, CBM |
| $Co_2MnSb$ | 6.01 (5.93[a]) | 0.42(HM)(0.49(HM)[a]) | 6.00 (6.00[a]) | Electrode | $\Delta_5$, $\Delta_1$ |
| HfIrSb | 6.33 (6.34[b]) | 0.87 (0.89)[b] | 0 | Spacer | $\Delta_2$, $\Delta_5$ & $\Delta_1$ |

[a]Ref:[1]
[b]Ref:[2,3]

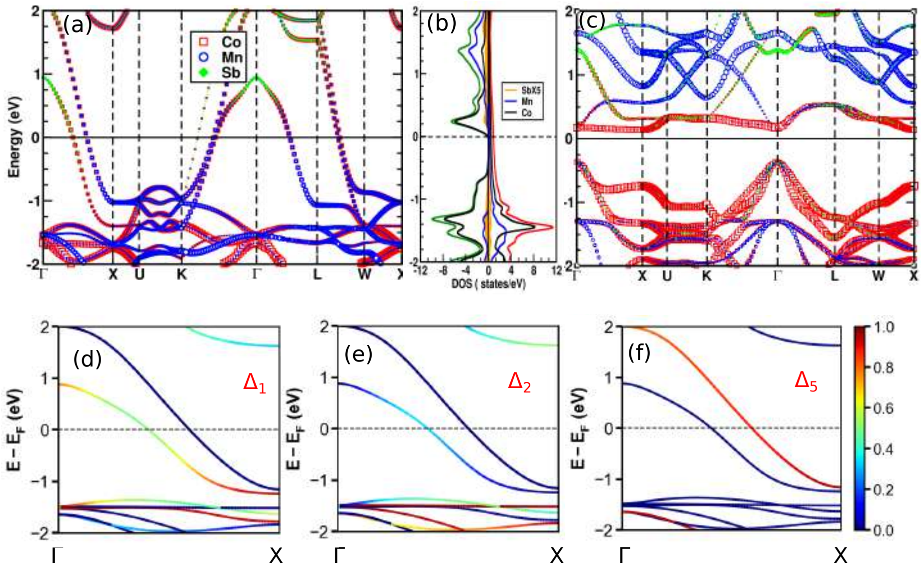


Figure S1. Panels (a), (c) show the majority and minority spin band structure, (b) depicts spin-polarized DOS of the bulk Co2MnSb structure. Panels (d), (e), and (f) display the orbital projected majority spin band structure along the Γ to X (Z) direction, where $\Delta_1$, $\Delta_2$, and $\Delta_5$ represent the (s, $p_z$, $d_{z^2}$), ($d_{xy}$, $d_{x^2-y^2}$), and ($p_x$, $p_y$, $d_{xz}$, $d_{yz}$) orbital characters, respectively.

Table S2. In plane strain, total and atomic magnetic moment ($\mu_T$ & $\mu_{Co}, \mu_{Mn}$) and spin polarization (in %) at $E_F$, calculated for the $Co_2MnSb$ bulk structure.

| In-plane strain (%) | c/a ratio | Magnetic moment (in $\mu_B$) | | | Spin-polarization (in %) |
|---|---|---|---|---|---|
| | | $\mu_T$ | $\mu_{Co}$ | $\mu_{Mn}$ | |
| -5 | 1.05 | 5.28 | 1 | 3.27 | -46 |
| -4 | 1.04 | 5.56 | 1.10 | 3.33 | -52 |
| -3 | 1.03 | 5.70 | 1.16 | 3.38 | -32 |
| -2 | 1.02 | 5.84 | 1.21 | 3.42 | -31 |
| -1 | 1.01 | 5.93 | 1.24 | 3.45 | 50 |
| 1 | 0.99 | 5.99 | 1.24 | 3.49 | 100 |
| 2 | 0.98 | 6.00 | 1.23 | 3.50 | 100 |
| 3 | 0.97 | 5.99 | 1.23 | 3.52 | 100 |
| 4 | 0.96 | 6.00 | 1.23 | 3.54 | 100 |
| 5 | 0.95 | 6.00 | 1.23 | 3.55 | 100 |

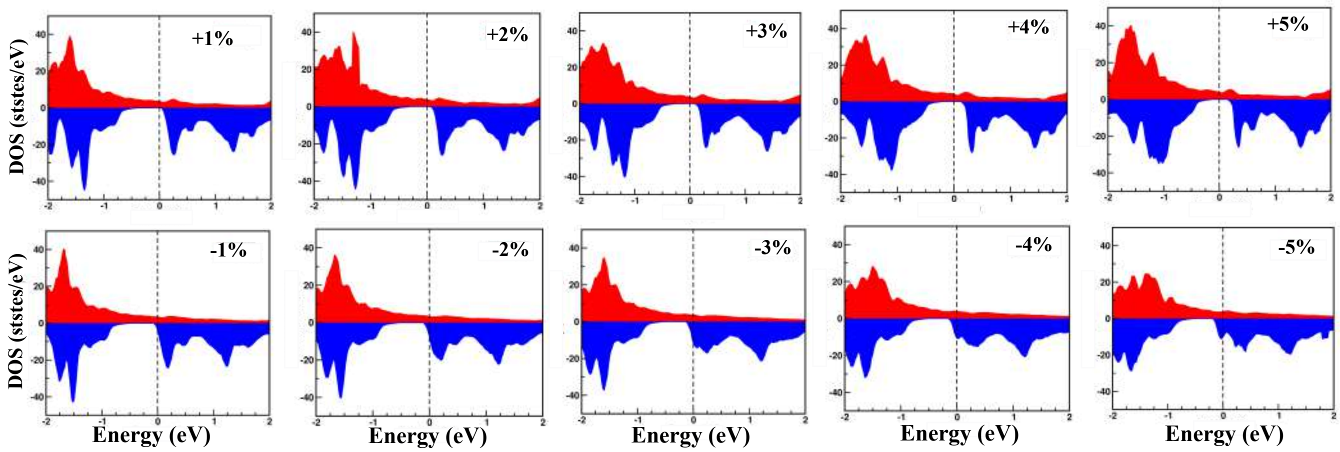


Figure S2. DOS of bulk $Co_2MnSb$ under biaxial strain (±5%) shown in two panels. The top panel corresponds to tensile strain, while the bottom panel corresponds to compressive strain.Here, red (blue) represent majority (minority) spin states.

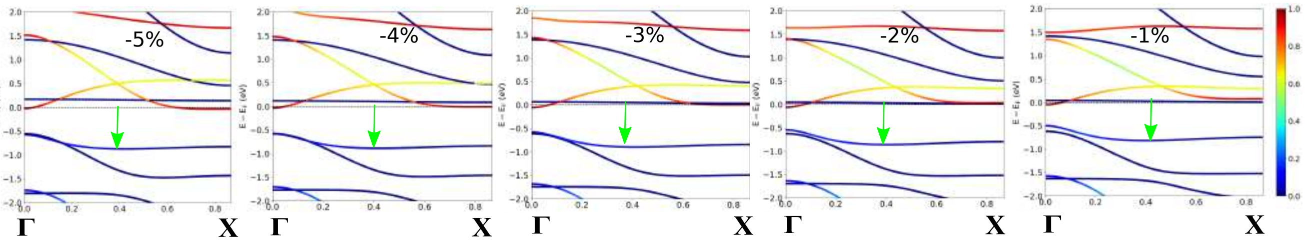


Figure S3. Effect of compressive bi-axial strain on the minority spin bands of the bulk $Co_2MnSb$. Here we have only shown the contribution from the $\Delta_1$ orbitals.

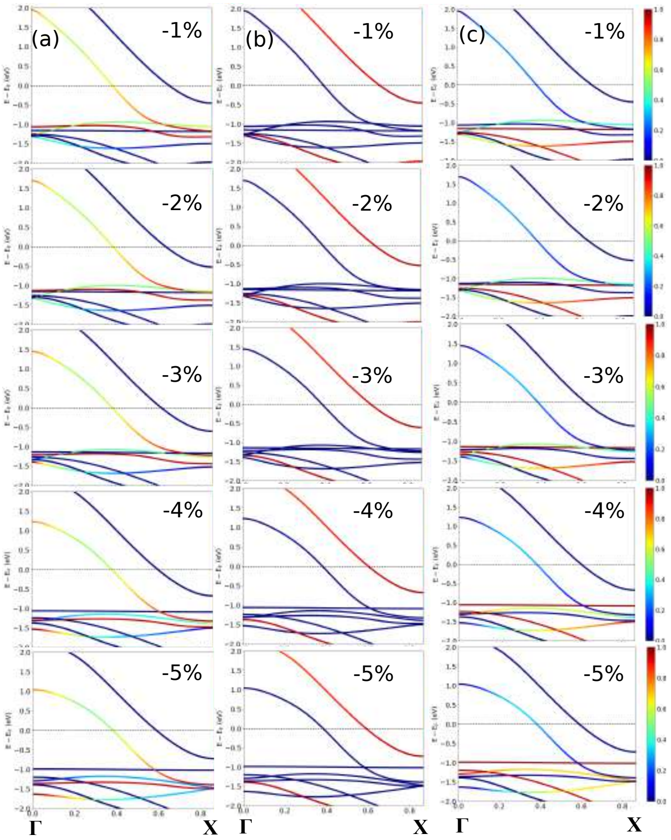


Figure S4. The majority spin band structure of bulk $Co_2MnSb$ under compressive biaxial strain (-1 to -5 %) is shown, where panels (a), (b), and (c) depict the orbital-projected majority spin band structure along the Γ to X (Z) direction. Here $\Delta_1$ (a), $\Delta_5$ (b), and $\Delta_2$ (c) represent the (s, $p_z$, $d_{z^2}$), ($p_x$, $p_y$, $d_{xz}$, $d_{yz}$), and ($d_{xy}$, $d_{x^2-y^2}$) orbital characters, respectively.

investigated their electronic and spin transport properties in conjunction with HfIrSb. In contrast, the Co-Co interface was neglected as it showed relatively poor surface SP.

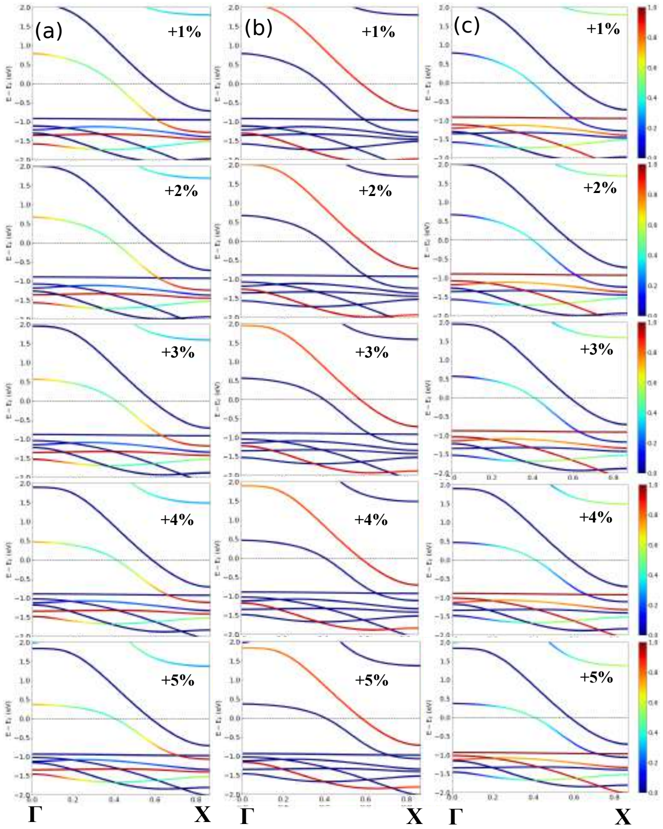


Figure S5. The majority spin band structure of bulk Co2MnSb under tensile bi-axial strain (1 to 5 %) is shown, where panels (a), (b), and (c) depict the orbital-projected majority spin band structure along the Γ to X (Z) direction. Here $\Delta_1$ (a), $\Delta_5$ (b), and $\Delta_2$ (c) represent the (s, $p_z$, $d_{z^2}$), ($p_x$, $p_y$, $d_{xz}$, $d_{yz}$), and ($d_{xy}$, $d_{x^2-y^2}$) orbital characters, respectively.

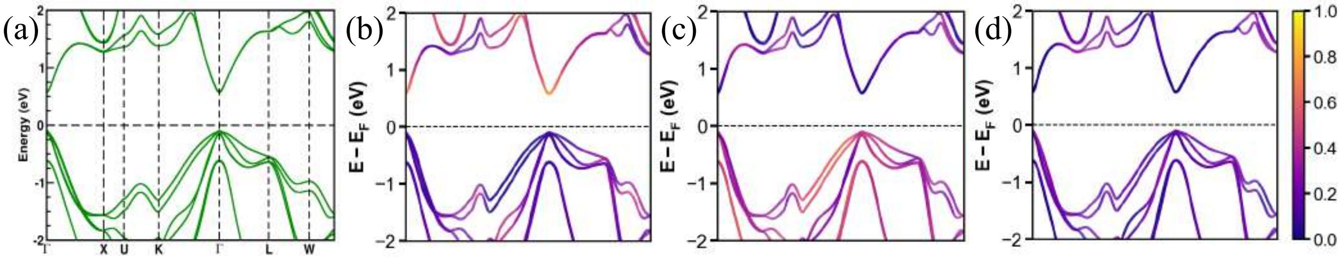


Figure S6. (a) The electronic band structure of HfIrSb, considering the influence of spin-orbit coupling interaction, is presented. Subsequent panels, (b), (c), and (d), illustrate the band structures resolved by orbital characteristics. Specifically, (b) represents (s, p$z$, d$z^2$) orbitals, (c) showcases (p$x$, p$y$, d$xz$, d$yz$) orbitals, while (d) displays (d$xy$, d$x^2 - y^2$) orbital contributions, respectively.

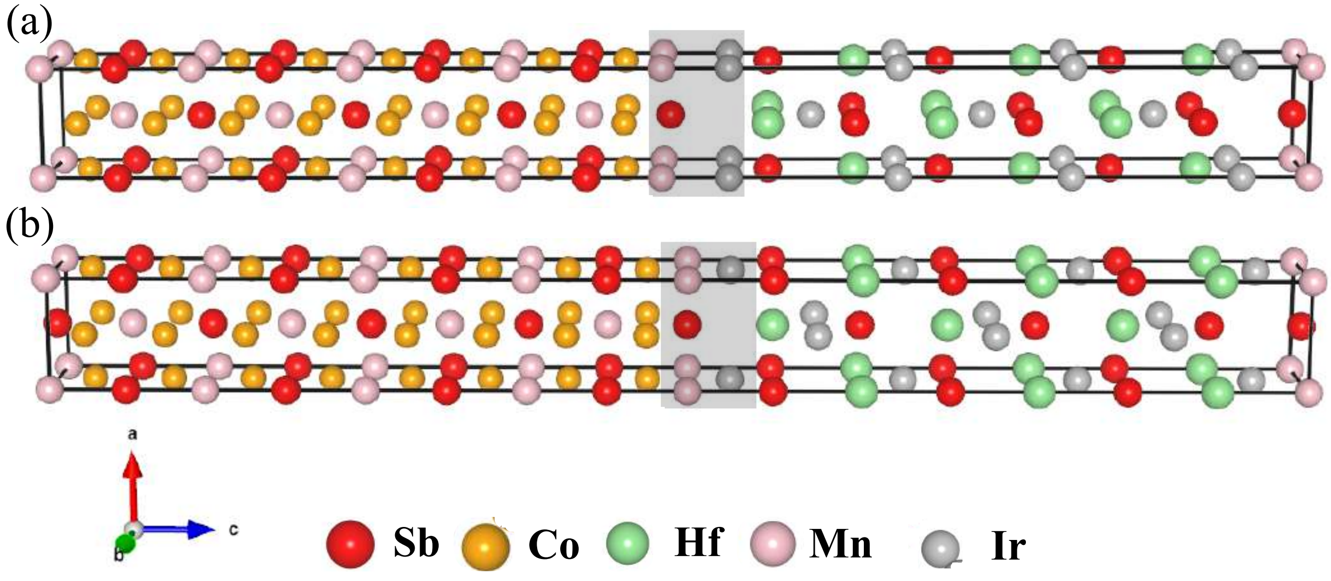


Figure S7. The schematic representation of $Co_2MnSb/HfIrSb$ heterostructure with a Mn-Sb/Ir interface: (a) Ir atoms are placed on the top of the Mn atoms (b) Ir atoms are placed at the hollow site . While the interfaces are symmetric, the heterostructure does not exhibit a perfect mirror symmetry about the Ir atom located at the center of the structure. The geometry was plotted using VESTA.

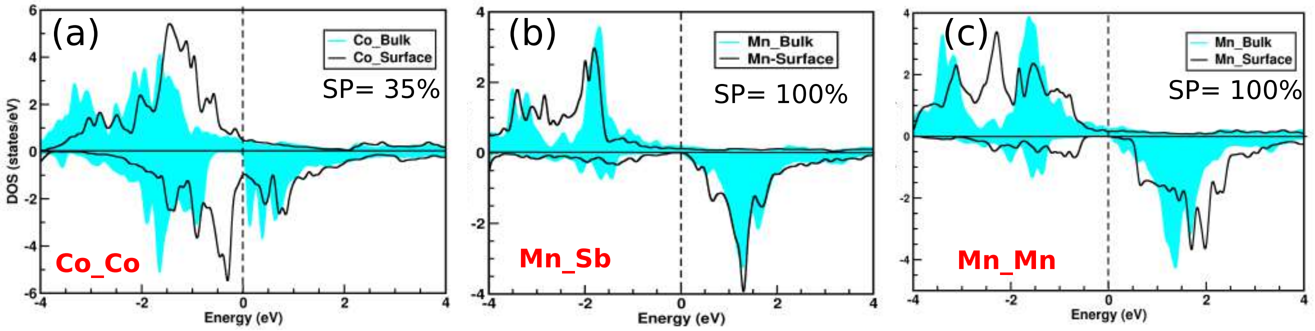


Figure S8. Atom projected density of states and respective values of spin polarization for different surface terminations along the (001) crystal orientation of $Co_2MnSb$.

Table S3. The surface free energy ( $\sigma_F$ in eV/Å$^2$), spin-polarization (SP in %) and magnetic moments (in $\mu_B$) the surface atoms (Mn atom for Mn-Sb and Mn-Mn termination and Co atom for Co-Co termination) of various terminations of $Co_2MnSb$ along (001) crystal orientations. The magnetic moments of the atoms inside the bulk are mentioned inside the bracket.

| Surface termination | $\sigma_F$ | Magnetic moment | SP |
|---|---|---|---|
| Mn-Sb | -4.1267 | 3.81 (3.46) | 100 |
| Co-Co | -4.1885 | 1.19 (1.31) | 35 |
| Mn-Mn | -4.0271 | 3.81, 3.85 (3.45) | 100 |

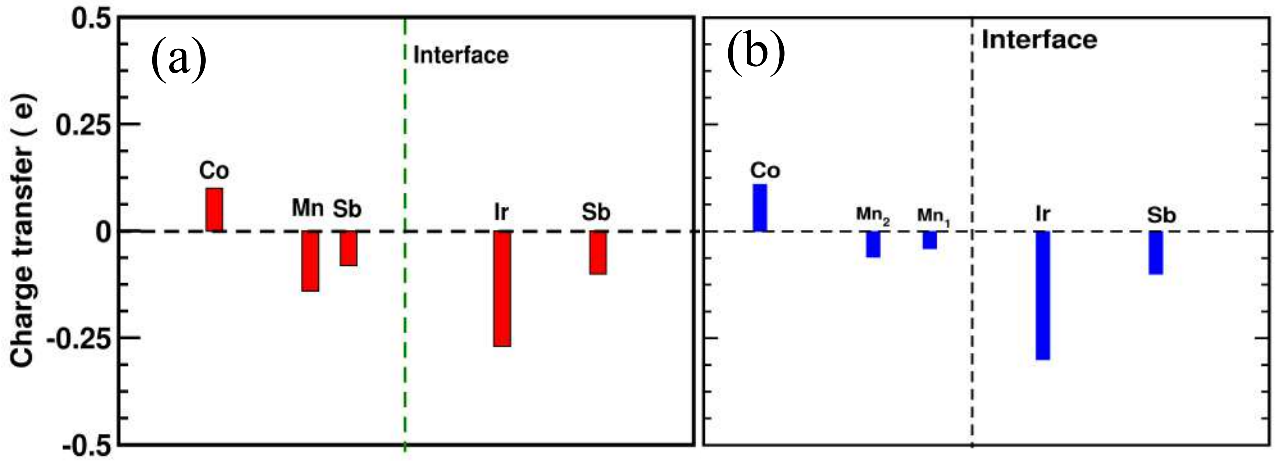


Figure S9. Charge transfer at the $Co_2MnSb$/HfIrSb interface as calculated from the Bader analysis: (a), (b) for Mn-Sb/Ir and Mn-Mn/Ir interface, respectively.

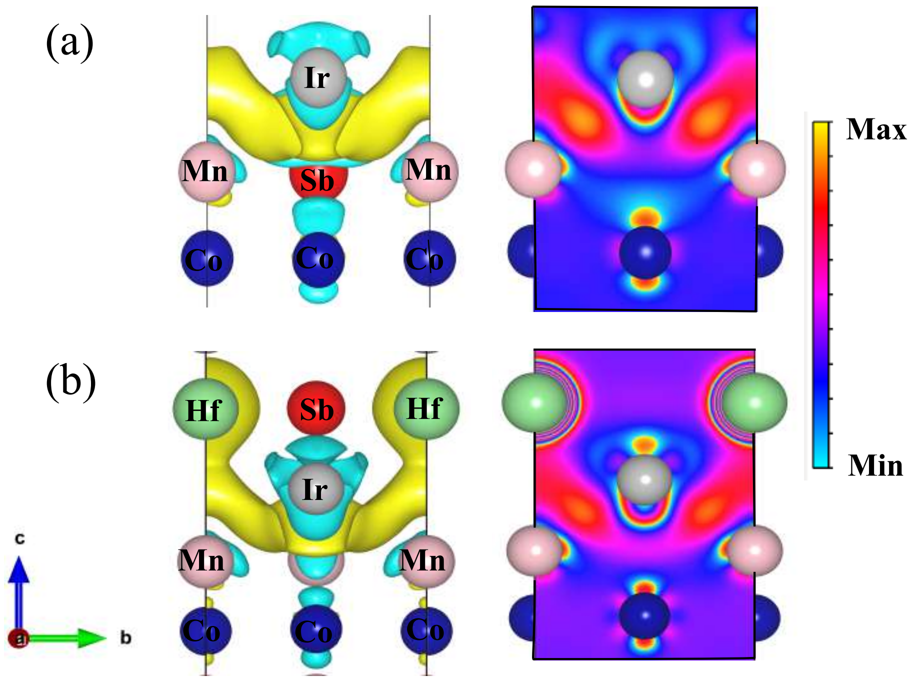


Figure S10. The charge density difference ($\Delta\rho$) of the heterostructure at the interface considering the spin-orbit coupling interaction, is plotted in two forms: a 3D visualization and a 2D visualization in the yz plane. Panels (a) and (b) show the $\Delta\rho$ at the Mn-Sb/Ir interface and Mn-Mn/Ir interface, respectively, where blue and yellow colors in the 3D visualization indicate negative and positive $\Delta\rho$, respectively. The isosurface value is set to 0.0003 e/A$^3$ for both cases.

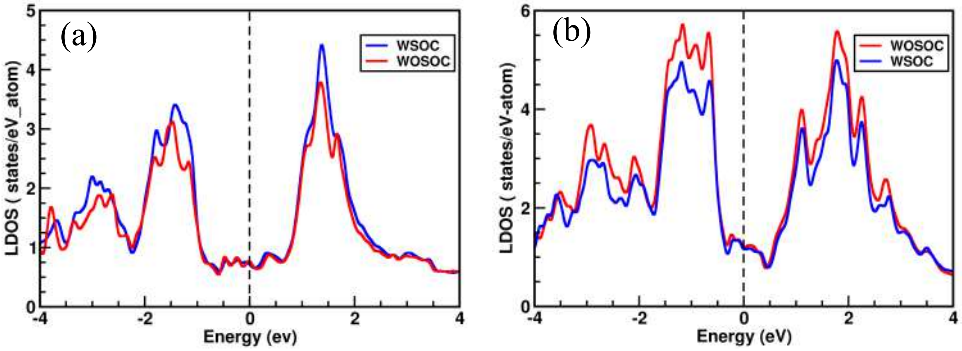


Figure S11. Comparison of total density of states of the interface atoms with and without considering the effects of spin-orbit-coupling for: (a) Mn-Sb/Ir , (b)Mn-Mn/Ir interface, respectively.

Table S4. Net charge transfer at the interface (in e), from Bader[5] analysis based on the VASP and Mulliken and Loewdin charge as obtained from LOBSTER package[6].

| Surface termination | Interface atom | Bader | Mulliken | Loewdin charge |
|---|---|---|---|---|
| Mn-Sb | Mn | -0.14 | -0.11 | -0.08 |
| | Sb | -0.08 | -0.24 | -0.15 |
| | Ir | -0.27 | -0.19 | -0.12 |
| Mn-Mn | $Mn_1$ | -0.03 | -0.07 | -0.06 |
| | $Mn_2$ | -0.06 | -.06 | -0.04 |
| | Ir | -0.29 | -0.43 | -0.33 |

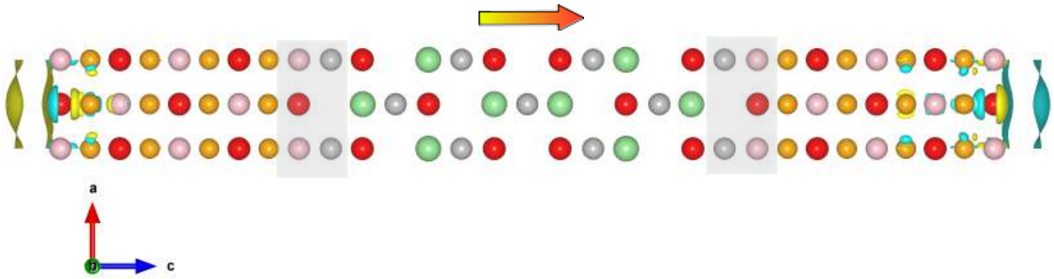


Figure S12. The variation in charge density ($\Delta\rho$) of $Co_2MnSb$/HfIrSb heterojunction, featuring the Mn-Sb/Ir interface, is displayed in the presence and absence of an external electric field. This representation illustrates $\Delta\rho = \Delta\rho^E - \Delta\rho$, under an external electric field (E) of 0.2 V/Å. The isosurface threshold is set at 0.001 eV/Å$^3$. The arrow at the top representing the direction of the externally applied electric field.

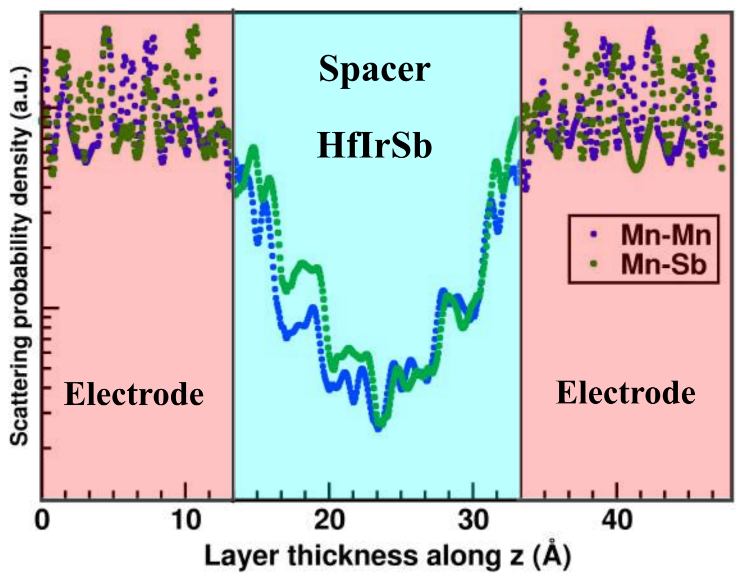


Figure S13. The absolute square of the right propagating scattering state wavefunctions at the Fermi energy ($E_F$) within the $Co_2MnSb$/HfIrSb heterojunction (with 13ML of spacer ) is depicted. The illustration showcases the penetration and decay of the wavefunction for two different interfaces, Mn-Sb/Ir and Mn-Mn/Ir, as a function of layer thickness.

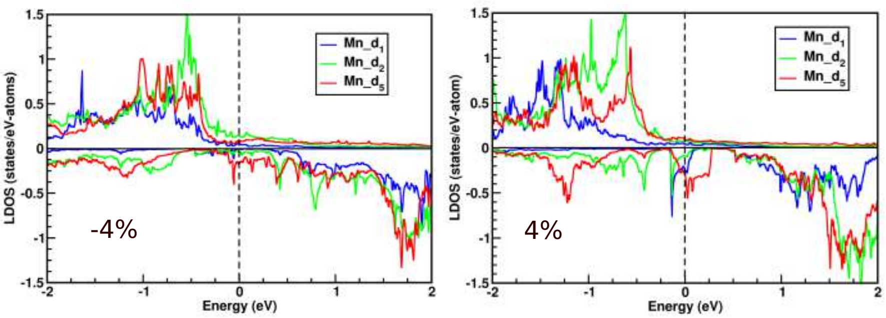


Figure S14. Orbital projected DOS of interfacial Mn atom under 4% compressive and tensile strain for Mn-Mn/Ir interface.Here, $d_1,\ d_5,\ d_2$ represents $d_{z^2},\ d_{xz,yz},\ and\ d_{x^2-y^2,xy}$ orbitals , respectively.

[1] Enamullah and S.-C. Lee, Journal of Alloys and Compounds **765**, 1055 (2018), ISSN 0925-8388.

[2] N. Arikan, G. DikiCi Yildiz, Y. G. Yildiz, and A. İyigör, Journal of Electronic Materials **49**, 3052 (2020), ISSN 1543-186X.

[3] M.-S. Lee, F. P. Poudeu, and S. D. Mahanti, Phys. Rev. B **83**, 159907 (2011).

[4] Y. Miura, H. Uchida, Y. Oba, K. Abe, and M. Shirai, Phys. Rev. B **78**, 064416 (2008).

[5] R. Bader (1990).

[6] R. Dronskowski and P. E. Bloechl, The Journal of Physical Chemistry **97**, 8617 (1993), ISSN 0022-3654.
